# Supplementary material for: K-Theory, D-Branes and Ramond-Ramond Fields
Source: arXiv:0812.0682 source file (2008-12-03)
Supplement: Supplementary file 1 [file appendixA.tex]

\newpage
\appendix{Clifford algebras and Spin manifolds}\label{appendixA}
\thispagestyle{plain}
